# Supplementary material for: Machine Learning-enhanced Receive Processing for MU-MIMO OFDM Systems
Source: arXiv:2106.16074 source file (2021-06-30)
Supplement: Supplementary file 1 [file appendix.tex]

\appendix
\subsection{Grouped-LMMSE equalizer}
\label{app:LMMSE}

We aim to find the \gls{LMMSE} matrix to equalize a group of \glspl{RE} that spans multiple subcarriers $f \in [F_b, F_e]$ and symbols $t \in [T_b, T_e]$, with $1 \leq F_b \leq F_e \leq N_f$ and $1 \leq T_b \leq T_e \leq N_t$.
Let us denote by $\widehat{\Hm}$ the estimated channel and by $\widetilde{\Hm}$ the estimation errors (assumed to have zero-mean).
The channel transfer function for that group can be written as
\begin{equation}
\yv_{f, t} = \LB \widehat{\Hm}_{f,t} + \widetilde{\Hm}_{f,t} \RB \xv_{f,t} + \nv_{f,t}, \quad \forall f \in [F_b, F_e], t \in [T_b, T_e].
\end{equation}
We denote by $\Wm_{f,t}, \;f \in [F_b, F_e], t \in [T_b, T_e]$ the \gls{LMMSE} matrix that minimizes
\begin{align}
\mathcal{L}(\Wm_{f,t}) 
& =\sum_{f'=F_b}^{F_e} \sum_{t'=T_b}^{T_e} \text{MSE}\LB  \xv_{f',t'}, \Wm_{f,t} \yv_{f',t'} \RB \\
&= \EE \LSB \sum_{f'=F_b}^{F_e} \sum_{t'=T_b}^{T_e} 
\LB\xv_{f', t'} - \Wm_{f,t} \yv_{f', t'} \RB
\LB\xv_{f', t'} - \Wm_{f,t} \yv_{f', t'} \RB\htp
 \RSB.
\end{align}
Therefore, $\Wm_{f,t}$ nulls the gradient 
\begin{equation}
\nabla_{\Wm_{f,t}} \mathcal{L}(\Wm_{f,t})
 = 2\Wm  \EE \LSB
\sum_{f'=F_b}^{F_e} \sum_{t'=T_b}^{T_e} 
 \yv_{f', t'} \yv_{f', t'}\htp  \RSB
- 2 \EE \LSB
\sum_{f'=F_b}^{F_e} \sum_{f'=T_b}^{T_e} 
\xv_{f', t'} \yv_{f', t'}\htp \RSB
\stackrel{!}{=} 0
\end{equation}
which leads to
\begin{align}
\Wm_{f,t} &= \LB \EE \LSB
\sum_{f'=F_b}^{F_e} \sum_{t'=T_b}^{T_e} 
 \xv_{f',t'} \yv_{f',t'}\htp  \RSB \RB
 \LB \EE \LSB
\sum_{f'=F_b}^{F_e} \sum_{t'=T_b}^{T_e} 
 \yv_{f',t'} \yv_{f',t'}\htp  \RSB \RB^{-1} \\
&=\LB 
\sum_{f'=F_b}^{F_e} \sum_{t'=T_b}^{T_e} 
 \Hm_{f',t'}^H  \RB
 \LB 
\sum_{f'=F_b}^{F_e} \sum_{t'=T_b}^{T_e} \LB
 \Hm_{f',t'} \Hm_{f',t'}\htp  
 + \EE \LSB \widetilde{\Hm}_{f',t'} \widetilde{\Hm}_{f',t'}\htp \RSB
 + \sigma^2\Id_{N_m}
 \RB \RB^{-1}.
\end{align}
